# Supplementary material for: Realizing Hopf Insulators in Dipolar Spin Systems
Source: arXiv:1901.08597 source file (2021-06-01)
Supplement: Supplementary file 1 [file supp.pdf]

# Supplemental Material: Realizing Hopf Insulators in Dipolar Spin Systems

Thomas Schuster,<sup>1</sup> Felix Flicker,<sup>1,2</sup> Ming Li,<sup>3</sup> Svetlana Kotochigova,<sup>3</sup> Joel E. Moore,<sup>1</sup> Jun Ye,<sup>4</sup> and Norman Y. Yao<sup>1</sup>

<sup>1</sup>*Department of Physics, University of California, Berkeley, California 94720 USA*

<sup>2</sup>*Rudolph Peierls Centre for Theoretical Physics, University of Oxford,  
Department of Physics, Clarendon Laboratory, Parks Road, Oxford, OX1 3PU, UK*

<sup>3</sup>*Department of Physics, Temple University, Philadelphia, Pennsylvania 19122, USA*

<sup>4</sup>*JILA, National Institute of Standards and Technology and Department of Physics,  
University of Colorado, Boulder, CO 80309, USA*

(Dated: January 23, 2019)

## CONTENTS

|                                                                 |   |
|-----------------------------------------------------------------|---|
| Effective Hamiltonian from the dipolar interaction              | 1 |
| Details of Floquet engineering                                  | 2 |
| Floquet engineering through a time-dependent chemical potential | 2 |
| Floquet engineering the Hopf Hamiltonian                        | 3 |
| Two-component scheme                                            | 3 |
| Even-odd modulation in $x$ - and $y$ -directions                | 4 |
| Truncation in the $z$ -direction                                | 4 |
| Details on numerics                                             | 5 |
| Calculating the Hopf invariant                                  | 5 |
| Finding the edge modes                                          | 5 |
| Details on AC polarizabilities for $z$ -direction modulation    | 5 |
| Details of the Experimental Implementation                      | 6 |
| References                                                      | 7 |

## EFFECTIVE HAMILTONIAN FROM THE DIPOLAR INTERACTION

We closely follow the discussion of Ref. [1]. The dipole-dipole interaction takes the form:

$$H_{\text{dd}}^{ij} = \frac{-\sqrt{6}}{4\pi\epsilon_0 R^3} \sum_{\Delta m_J = -2}^2 C_{-\Delta m_J}^2(\theta, \phi) T_{\Delta m}^2(\mathbf{d}^{(i)}, \mathbf{d}^{(j)}). \quad (1)$$

Here the displacement between lattice sites  $i$  and  $j$ , parameterized in spherical coordinates as  $(R, \theta, \phi)$ . The dipole moment operator  $\mathbf{d}^{(i)} = (d_-^{(i)}, d_z^{(i)}, d_+^{(i)})$  is a rank-1 spherical tensor, which acts on the rotational states of the molecule at lattice site  $i = \mathbf{v}, \alpha$  and changes the molecule's magnetic quantum number by  $(-1, 0, +1)$ . The spherical harmonics  $C_{-\Delta m}^2(\theta, \phi)$  have normalization according to Ref. [2], and  $T_{\Delta m}^2$  is the unique rank-2 spherical tensor generated from the dipole operators  $\mathbf{d}^{(i)}$  and  $\mathbf{d}^{(j)}$ :  $T_{\pm 2}^2 = d_{\pm}^{(i)} d_{\pm}^{(j)}$ ,  $T_{\pm 1}^2 = (d_{\pm}^{(i)} d_z^{(j)} + d_z^{(i)} d_{\pm}^{(j)})/\sqrt{2}$ ,  $T_0^2 = (d_{\pm}^{(i)} d_{\mp}^{(j)} + 2d_z^{(i)} d_z^{(j)} + d_{\mp}^{(i)} d_{\pm}^{(j)})/\sqrt{6}$ , with  $d_{\pm} = \mp(d_x \pm id_y)/\sqrt{2}$ .

When the dipole-dipole interaction is weak compared to the splitting between rotational levels, this interaction gives rise to an effective Hamiltonian in the restricted hard-core boson Hilbert space (introduced in the main text). The hoppings of this Hamiltonian are calculated as  $t_{ij} = \langle 0_i, 1_j | H_{\text{dd}}^{ij} | 1_i, 0_j \rangle$ . Our choice  $|1_A\rangle = |1, M_A = 0\rangle$  and  $|1_B\rangle = |1, M_B = 1\rangle$  guarantees that only  $\Delta m_J = 0$  terms will contribute to intra-sublattice hoppings, and only

$\Delta m_J = 1$  terms to inter-sublattice hoppings. Restoring unit cell/sublattice indices, we calculate

$$\begin{aligned} t_{\mathbf{R}}^{AA} &= -\frac{2 d_{00}^2}{4\pi\epsilon_0 R^3} C_0^2(\theta, \phi) = -\frac{d_{00}^2}{4\pi\epsilon_0} \frac{3 \cos^2(\theta) - 1}{R^3} \\ t_{\mathbf{R}}^{BB} &= \frac{d_{01}^2}{4\pi\epsilon_0 R^3} C_0^2(\theta, \phi) = \frac{d_{01}^2}{8\pi\epsilon_0} \frac{3 \cos^2(\theta) - 1}{R^3} \\ t_{\mathbf{R}}^{AB} &= \frac{\sqrt{3} d_{00} d_{01}}{4\pi\epsilon_0 R^3} C_{-1}^2(\theta, \phi) = -\frac{3 d_{00} d_{01}}{4\sqrt{2}\pi\epsilon_0} \frac{\cos(\theta) \sin(\theta)}{R^3} e^{i\phi}. \end{aligned} \quad (2)$$

where  $(R, \theta, \phi)$  again parameterizes the displacement between sites in spherical coordinates, which equals  $\mathbf{r}$  for intra-sublattice hoppings and  $\mathbf{r} + b\hat{\mathbf{z}}$  for inter-sublattice hoppings, and  $d_{00} = \langle 1, 0 | d_z | 0, 0 \rangle$  and  $d_{01} = \langle 1, \pm 1 | d_{\pm} | 0, 0 \rangle$ . This reproduces the hoppings of the main text with  $C^{AA} = \frac{d_{00}^2}{4\pi\epsilon_0}$ ,  $C^{BB} = \frac{d_{01}^2}{8\pi\epsilon_0}$ ,  $C^{AB} = \frac{3 d_{00} d_{01}}{4\sqrt{2}\pi\epsilon_0}$ . The presence of a DC electric field will mix the  $|0, 0\rangle$  and  $|1, 0\rangle$  states, and give rise to additional long-range density-density *interactions* in the hard-core boson model. We neglect these in our study of the single-particle physics of the Hopf insulator.

## DETAILS OF FLOQUET ENGINEERING

We first discuss Floquet engineering using a time-dependent chemical potential generally, based largely on Ref. [3], before proceeding to its use in our proposal.

### Floquet engineering through a time-dependent chemical potential

Here we review the discussion of Ref. [3], generalized to include sublattices and complex hoppings. The system's time-dependent Hamiltonian takes the form

$$\hat{H}(t) = \frac{1}{2} \sum_{\substack{\mathbf{v}, \mathbf{r} \neq \mathbf{0}, \\ \alpha, \beta}} [t_{\mathbf{r}}^{\alpha\beta} a_{\mathbf{v}+\mathbf{r}, \alpha}^\dagger a_{\mathbf{v}, \beta} + h.c.] + \sum_{\mathbf{v}, \alpha} f_{\mathbf{v}}^\alpha(t) a_{\mathbf{v}, \alpha}^\dagger a_{\mathbf{v}, \alpha}, \quad (3)$$

where  $f_{\mathbf{r}}(t)$  is periodic in  $t$  with period  $T$ . To calculate the effect of the driving, we move into a rotating frame, defining the unitary

$$U(t) = \exp \left[ -i \int_0^t dt' \frac{1}{2} \sum_{\mathbf{r}} f_{\mathbf{r}}(t') \sigma_{\mathbf{r}}^z \right], \quad (4)$$

the rotated wavefunction

$$|\Psi'(t)\rangle = U^\dagger(t) |\Psi(t)\rangle, \quad (5)$$

and the rotated Hamiltonian

$$\begin{aligned} H'(t) &= U^\dagger(t) H(t) U(t) - i U^\dagger(t) \dot{U}(t) \\ &= \frac{1}{2} \sum_{\substack{\mathbf{v}, \mathbf{r} \neq \mathbf{0}, \\ \alpha, \beta}} \left[ \exp \left[ -i \int_0^t dt' (f_{\mathbf{v}+\mathbf{r}}^\alpha(t') - f_{\mathbf{v}}^\beta(t')) \right] t_{\mathbf{r}}^{\alpha\beta} a_{\mathbf{v}+\mathbf{r}, \alpha}^\dagger a_{\mathbf{v}, \beta} + h.c. \right]. \end{aligned} \quad (6)$$

Next, we perform a high-frequency expansion in the rotated Hamiltonian by replacing all oscillating quantities with their average over a period, valid if  $1/T \gg |t_{\mathbf{r}}^{\alpha\beta}|$ . This gives an effective Hamiltonian

$$H^{\text{eff}} = \frac{1}{2} \sum_{\substack{\mathbf{v}, \mathbf{r} \neq \mathbf{0}, \\ \alpha, \beta}} [\beta_{\mathbf{v}+\mathbf{r}, \mathbf{v}}^{\alpha\beta} t_{\mathbf{r}}^{\alpha\beta} a_{\mathbf{v}+\mathbf{r}, \alpha}^\dagger a_{\mathbf{v}, \beta} + h.c.] + \sum_{\mathbf{v}, \alpha} f_{\mathbf{v}}^\alpha(t) a_{\mathbf{v}, \alpha}^\dagger a_{\mathbf{v}, \alpha}, \quad (7)$$

with static chemical potential

$$\mu_{\mathbf{v}}^{\alpha} = \frac{1}{T} \int_0^T dt f_{\mathbf{v}}^{\alpha}(t) \quad (8)$$

and hoppings suppressed by the ‘damping coefficients’,

$$\begin{aligned} \beta_{\mathbf{v}+\mathbf{r},\mathbf{v}}^{\alpha\beta} &= \frac{1}{T} \int_0^T dt \exp \left[ -i \int_0^t dt' (f_{\mathbf{v}+\mathbf{r}}^{\alpha}(t') - f_{\mathbf{v}}^{\beta}(t')) \right] \\ &= \frac{1}{T} \int_0^T dt \left( \cos \left[ \int_0^t dt' (f_{\mathbf{v}+\mathbf{r}}^{\alpha}(t') - f_{\mathbf{v}}^{\beta}(t')) \right] - i \sin \left[ \int_0^t dt' (f_{\mathbf{v}+\mathbf{r}}^{\alpha}(t') - f_{\mathbf{v}}^{\beta}(t')) \right] \right). \end{aligned} \quad (9)$$

Generally  $\beta_{\mathbf{v}+\mathbf{r},\mathbf{v}}^{\alpha\beta}$  can be complex. We will always choose  $f_{\mathbf{v}}^{\alpha}(t)$  to be an even function of  $t$ , in which case the imaginary part vanishes and we have

$$\beta_{\mathbf{v}+\mathbf{r},\mathbf{v}}^{\alpha\beta} = \frac{1}{T} \int_0^T dt \cos \left[ \int_0^t dt' (f_{\mathbf{v}+\mathbf{r}}^{\alpha}(t') - f_{\mathbf{v}}^{\beta}(t')) \right]. \quad (10)$$

This ensures that  $\beta_{\mathbf{v}+\mathbf{r},\mathbf{v}}^{\alpha\beta}$  modulates only the hopping magnitude, and not the phase.

To preserve translational invariance, the damping coefficients must depend only on the displacement  $\mathbf{r}$ , and not the lattice site  $\mathbf{v}$ :  $\beta_{\mathbf{v}+\mathbf{r},\mathbf{v}}^{\alpha\beta} = \beta_{\mathbf{r}}^{\alpha\beta}$ . This imposes a number of constraints on the Floquet modulation  $f_{\mathbf{v}}^{\alpha}(t)$ . For intra-sublattice hoppings ( $\alpha = \beta$ ), one requires that  $\cos \left[ \int_0^t dt' (f_{\mathbf{v}+\mathbf{r}}^{\alpha}(t') - f_{\mathbf{v}}^{\alpha}(t')) \right]$  be independent of  $\mathbf{v}$ . There are two ways to achieve this: 1) with a ‘gradient’ modulation  $f_{\mathbf{v}}^{\alpha}(t)$  linear in  $\mathbf{v}$ , and 2) with an ‘even-odd’ modulation  $f_{\mathbf{v}}^{\alpha}(t) = f^{\alpha}(-1)^{s_x v_x + s_y v_y + s_z v_z}$ ,  $s_i \in \{0, 1\}$ . The latter is possible because we restricted ourselves to the cosine term of Eq. (9), which is even in  $f$  and thus requires only the absolute value of  $f_{\mathbf{v}+\mathbf{r}}^{\alpha}(t') - f_{\mathbf{v}}^{\alpha}(t')$  to be independent of  $\mathbf{v}$ . For inter-sublattice hoppings, one requires that  $\cos \left[ \int_0^t dt' (f_{\mathbf{v}+\mathbf{r}}^A(t') - f_{\mathbf{v}}^B(t')) \right]$  be independent of  $\mathbf{v}$ . This requires that the sublattice modulations differ only by a *position-independent* function of time,

$$\begin{aligned} f_{\mathbf{v}}^A(t) &= f_{\mathbf{v}}(t) \\ f_{\mathbf{v}}^B(t) &= f_{\mathbf{v}}(t) + f_{SL}(t). \end{aligned} \quad (11)$$

Altogether, we have shown that translational invariance requires that the modulation take the form  $f_{\mathbf{v}}^A(t) = f_{\mathbf{v}}(t)$ ,  $f_{\mathbf{v}}^B(t) = f_{\mathbf{v}}(t) + f_{SL}(t)$ , with two possibilities for the position-dependence of  $f_{\mathbf{v}}(t)$ . This gives rise to damping coefficients

$$\begin{aligned} \beta_{\mathbf{r}}^{AA} &= \frac{1}{T} \int_0^T dt \cos \left[ \int_0^t dt' (f_{\mathbf{v}+\mathbf{r}}(t') - f_{\mathbf{v}}(t')) \right] \\ \beta_{\mathbf{r}}^{BB} &= \beta_{\mathbf{r}}^{AA} \\ \beta_{\mathbf{r}}^{AB} &= \frac{1}{T} \int_0^T dt \cos \left[ \int_0^t dt' (f_{\mathbf{v}+\mathbf{r}}(t') - f_{\mathbf{v}}(t') - f_{SL}(t')) \right]. \end{aligned} \quad (12)$$

which may be different for inter-sublattice and intra-sublattice hoppings.

## Floquet engineering the Hopf Hamiltonian

### Two-component scheme

In our proposal, Floquet engineering is utilized to two distinct effects: *i*) to modulate the strength of even vs. odd hoppings in the  $x$ - and  $y$ -directions, and *ii*) to truncate hoppings in the  $z$ -direction from power law (the bare dipole-dipole interactions  $t_{\mathbf{r}}^{\alpha\beta}$ ) to effectively nearest-neighbor. To do this we take the modulation amplitude to have two components that oscillate at *different frequencies*,

$$f_{\mathbf{r}}^{\alpha}(t) = f_{\mathbf{r}}^{xy,\alpha}(t) + f_{\mathbf{r}}^{z,\alpha}(t), \quad (13)$$

where  $f_{\mathbf{r}}^{xy,\alpha}(t)$  is periodic with frequency  $\Omega^{xy} \equiv 2\pi/T^{xy}$  and  $f_{\mathbf{r}}^{z,\alpha}(t)$  is periodic with frequency  $\Omega^z \equiv 2\pi/T^z$ . We require the frequencies  $\Omega^{xy}$  and  $\Omega^z$  be on very different scales, namely  $\Omega^{xy} \gg \Omega^z$  or  $\Omega^{xy} \ll \Omega^z$ , in order for the effects of these two components to be independent. (Without this, the Floquet engineering will in fact break translational invariance and double the size of the unit cell.) If this holds, then  $\beta_{\mathbf{v}}^{\alpha\beta}$  factorizes into the product of the two components' individual damping coefficients,

$$\beta_{\mathbf{v}}^{\alpha\beta} = \beta_{\mathbf{v}}^{xy,\alpha\beta} \beta_{\mathbf{v}}^{z,\alpha\beta}, \quad (14)$$

$$\beta_{\mathbf{r}}^{xy,\alpha\beta} = \frac{1}{T^{xy}} \int_0^{T^{xy}} dt \cos \left[ \int_0^t dt' (f_{\mathbf{v}+\mathbf{r}}^{xy,\alpha}(t') - f_{\mathbf{v}}^{xy,\beta}(t')) \right] \quad (15)$$

$$\beta_{\mathbf{r}}^{z,\alpha\beta} = \frac{1}{T^z} \int_0^{T^z} dt \cos \left[ \int_0^t dt' (f_{\mathbf{v}+\mathbf{r}}^{z,\alpha}(t') - f_{\mathbf{v}}^{z,\beta}(t')) \right]. \quad (16)$$

*Even-odd modulation in  $x$ - and  $y$ -directions*

The Floquet modulation in the  $x$ - and  $y$ - directions uses the even-odd modulation previously introduced, with  $s_x = s_y = 1, s_z = 0$ . Specifically, we take

$$\begin{aligned} f_{\mathbf{v}}^{xy}(t) &= \frac{1}{2}(-1)^{v_x+v_y} \Omega^{xy} g^{xy} \cos(\Omega^{xy} t) \\ f_{SL}^{xy}(t) &= \Omega^{xy} g_{SL}^{xy} \cos(\Omega^{xy} t). \end{aligned} \quad (17)$$

The two parameters  $g^{xy}$  and  $g_{SL}^{xy}$  give independent control over the ratios of even to odd hoppings for inter- and intra-sublattice hoppings. Performing the integral inside Eq. (15) and using  $\frac{1}{T} \int_0^T dt \cos[g \sin(2\pi t/T)] = \frac{1}{2\pi} \int_0^{2\pi} dx \cos[g \sin(x)] = J_0(g)$ , where  $J_0(g)$  is a Bessel function of the first kind, gives damping coefficients

$$\begin{aligned} \beta_{\mathbf{r}}^{xy,AA} &= \begin{cases} J_0(g^{xy}) & r_x + r_y = \text{odd} \\ 1 & r_x + r_y = \text{even} \end{cases} \\ \beta_{\mathbf{r}}^{xy,AB} &= \begin{cases} J_0(g^{xy} + g_{SL}^{xy}) & r_x + r_y = \text{odd} \\ J_0(g_{SL}^{xy}) & r_x + r_y = \text{even}. \end{cases} \end{aligned} \quad (18)$$

*Truncation in the  $z$ -direction*

Our second use of Floquet modulation is to truncate the hoppings to effectively nearest-neighbor in the  $z$ -direction, similar to Ref. [3]. We take  $f_{\mathbf{v}}^z(t)$  to be a gradient in the  $z$ -direction,

$$\begin{aligned} f_{\mathbf{v}}^z(t) &= v_z \Omega^z g^z(\Omega^z t) \\ f_{SL}^z(t) &= \Omega^z g_{SL}^z(\Omega^z t) \end{aligned} \quad (19)$$

which gives,

$$\beta_{\mathbf{r}}^{z,AA} = \frac{1}{2\pi} \int_0^{2\pi} dx \cos \left[ r_z \int_0^x dx' g^z(x') \right] \quad (20)$$

$$\beta_{\mathbf{r}}^{z,AB} = \frac{1}{2\pi} \int_0^{2\pi} dx \cos \left[ \int_0^x dx' [r_z g^z(x') - g_{SL}^z(x')] \right]. \quad (21)$$

These can be evaluated numerically once the functions  $g^z(x), g_{SL}^z(x)$  are chosen. Ref. [3] showed that these can be tuned to give hoppings that are effectively nearest-neighbor in the  $z$ -direction, at the cost of some loss of magnitude of the nearest-neighbor  $|r_z| = 1$  hopping.

## DETAILS ON NUMERICS

### Calculating the Hopf invariant

In numerically computing the Hopf invariant, we truncate all infinite sums over  $\mathbf{r}$  by only including hoppings to sites at most  $R$  unit cells away in each direction, so  $t_{\mathbf{r}}^{\alpha\beta}$  for  $|r_i| \leq R$ ,  $i = \{x, y, z\}$ . We see quantitative agreement of the band gap within 1% for all  $8 \leq R \leq 32$ . The Hopf integral is computed by evaluating  $\mathbf{j}(\mathbf{k})$  from  $\hat{\mathbf{n}}(\mathbf{k})$  on an  $N \times N \times N$  grid in momentum space and solving  $\nabla \times \mathbf{A}(\mathbf{k}) = \mathbf{j}(\mathbf{k})$  in the inverse Fourier domain [4]. The invariant converges quickly to 1 as  $N$  becomes large, e.g.  $h - 1 \approx 10^{-6}$  at  $N = 70, R = 4$ .

### Finding the edge modes

The spectrum is calculated via exact diagonalization of the hybrid real/momentum-space Hamiltonian  $H_{xx'}(k_y, k_z) = \sum_{\mathbf{r}} t_{\mathbf{r}}^{\alpha\beta} \delta_{r_x=x-x'}$  for the effective Hamiltonian hoppings, truncated at range  $R = 4$ . Sharp edge modes are calculated for a lattice with  $N_s = 80$  unit cells in the  $x$ -direction with open boundary conditions. The symmetry-breaking perturbation is chosen as a site-dependent (but sublattice-independent) chemical potential  $\mu_{\mathbf{v}} \mathbb{1}$  localized on the two unit cells  $\mathbf{v}$  nearest each edge. Adiabatic edge modes are calculated on a lattice with  $N_a = 160$  unit cells in the  $x$ -direction, also with open boundary conditions. The hoppings are taken to be constant throughout the lattice, while an  $x$ -dependent 'staggered' chemical potential  $\mu_x \sigma_z$  tunes the Hamiltonian between the trivial phase at each end of the lattice and the Hopf insulator phase in the center. Specifically, we take

$$\mu_x = \begin{cases} 0 & 0 < x \leq 48 \\ \frac{3}{2} \frac{x-48}{20} & 48 < x \leq 68 \\ \frac{3}{2} & 68 < x \leq N_a/2 \\ \mu_{N_a-x} & N_a/2 < x \leq N_a \end{cases} . \quad (22)$$

This has two edge mode regions of width 20. After calculating the matrix  $H_{xx'}(k_y, k_z)$  for a given  $k_y, k_z$ , its eigenvectors and eigenvalues are found via exact diagonalization. The edge modes are determined by calculating the mean position  $\langle x \rangle$  for each mode - those with positions far from the center are edge modes. For Fig. 3 of the main text this was repeated for 400 evenly-spaced values of  $k_y$  with  $k_z = 0$ .

## DETAILS ON AC POLARIZABILITIES FOR $z$ -DIRECTION MODULATION

To effectively implement the Floquet modulation along  $z$ -direction, we opt to use circularly polarized light near a narrow transition which allows light shifts to be precisely controlled by the detuning from the transition. For the  $^{40}\text{K}^{87}\text{Rb}$  system, we choose the dipole-forbidden transition  $|X^1\Sigma^+, v=0, J=1, m_J\rangle \rightarrow |b^3\Pi_{0^+}, v=0, J=2, m_J+1\rangle$  with 1028.7 nm [5]  $\sigma^+$  light where  $m_J = 0$  for the A sublattice and 1 for the B sublattice. With relatively weak laser intensity (on the order of  $\text{W}/\text{cm}^2$ ), the light shift can be characterized by the AC polarizability of the molecular state of interest. The polarizability is calculated from two different contributions. The first and more important contribution comes from the resonant transition which has a strong dependence on the detuning, and the second contribution comes from all other transitions that has negligible dependence on the detuning in the range we are interested in. Here we assume the detuning is much larger than the spacings between  $|X^1\Sigma^+, v=0, J=1, m_J\rangle$  states with  $m_J = 0$  and  $\pm 1$ , and these spacings are much larger than the light shifts.

To characterize the contributions from the resonant transition, we follow the recipe in Refs. [6–8]. The generally complex dynamic polarizability for alkali-metal molecule in a rovibrational state of the ground  $X^1\Sigma^+$  potential is given by

$$\alpha(h\nu, \hat{\varepsilon}) = \frac{1}{\varepsilon_0 c} \sum_f \frac{E_f - E_i - i\hbar\gamma_f/2}{(E_f - E_i - i\hbar\gamma_f/2)^2 - (h\nu)^2} |f|d\hat{R} \cdot \hat{\varepsilon}|i\rangle|^2 . \quad (23)$$

$\hat{\varepsilon}$  and  $\nu$  are the polarization vector and the frequency of the light, respectively,  $c$  is the speed of light,  $\varepsilon_0$  is the electric constant,  $\hat{R}$  is the orientation of the interatomic axis, and  $d$  is the dipole operator.  $i$  denotes the rovibrational state

$|i\rangle$  of interest with energy  $E_i$  in the ground  $X^1\Sigma^+$  potential, and the summation over  $f$  denotes the summation over all rovibrational states  $|f\rangle$  other than  $i$  with energies  $E_f$  in all electronic potentials, and  $\gamma_f$  describe the natural linewidths of  $|f\rangle$ .

When the laser frequency is very close to the narrow dipole-forbidden transition, the most significant contribution comes from that transition which has a pole at the resonant frequency and weakens as the inverse function of the detuning. We treat all transitions from  $|X^1\Sigma^+, v=0, J=1, m_J\rangle$  to rovibrational states in the  $b^3\Pi_{0+}$  potential using Eq. (23). The largest contribution by far comes from the transition to the excited  $v=0$  state due to the similarity of its radial wavefunction to the ones in the ground potential. We use the experimentally adjusted potential energy curves for both the excited  $b^3\Pi_{0+}$  state [9] and the ground  $X^1\Sigma^+$  state [10], and a spin-orbit modified transition dipole moment between them [11]. Since the natural linewidths of the lowest rovibrational states in the  $b^3\Pi_{0+}$  potential are much smaller (on the order of kHz [5]) than the detunings we are interested in (on the order of GHz), we take  $\gamma_f = 0$ .

The background contributions from all other transitions have negligible frequency dependence close to the 1028.7 nm transition due to the large detunings from the corresponding excited states. Thus we treat the background polarizabilities as constants throughout the detuning range. We use the method in Ref. [12] with experimentally determined electronic parallel and perpendicular polarizabilities [13] to calculate the background polarizabilities at 1064 nm and assume them to be the same near the 1028.7 nm transition. More specifically, we use  $\alpha_{\parallel}/h = 10.0(3) \times 10^{-5}$  MHz/(W/cm<sup>2</sup>) and  $\alpha_{\perp}/h = 3.3(1) \times 10^{-5}$  MHz/(W/cm<sup>2</sup>) determined for the wavelength of 1064 nm and obtain the background polarizabilities  $\alpha_{bg,|1,0\rangle}/h = 4.64 \times 10^{-5}$  MHz/(W/cm<sup>2</sup>) and  $\alpha_{bg,|1,1\rangle}/h = 5.98 \times 10^{-5}$  MHz/(W/cm<sup>2</sup>) for  $\sigma^+$  polarization.

Finally, we add the two parts together to arrive at the total AC polarizabilities shown in Fig. 3 of the main text.

## DETAILS OF THE EXPERIMENTAL IMPLEMENTATION

Here we review the experimental implementation of our proposal in lattices of  $^{40}\text{K}^{87}\text{Rb}$  in more detail. The molecule  $^{40}\text{K}^{87}\text{Rb}$  has a rotational splitting  $\Delta = 2.2$  GHz and a measured dipolar interaction strength  $\sim 50$  Hz when trapped in a 3D optical lattice with 1064nm light [14]. Our proposed external DC electric and magnetic fields are oriented in the  $z$ -direction with strengths 1650 V/m and -490 G respectively. The  $x$ - and  $y$ - sublattices are formed with light polarized in the  $z$ -direction of intensity  $I_{x,y} = .5$  kW/cm<sup>2</sup>, while the  $z$ -lattice is formed with  $x$ -polarized light of intensities  $I_A = .43$  kW/cm<sup>2</sup> and  $I_B = .54$  kW/cm<sup>2</sup>. Energy levels for this configuration are calculated as in Ref. [13]. They feature the desired degeneracy between the  $|1,0\rangle_A \rightarrow |0,0\rangle_A$  and  $|1,1\rangle_B \rightarrow |0,0\rangle_B$  transitions, with an energy gap  $\gtrsim 5$  kHz to all other rotational transitions. We choose a lattice distance 1.01 in the  $z$ -direction (in units of the  $xy$ -plane lattice spacing) and a vertical spacing 0.66 between the sublattices. A chemical potential of  $\mu^A - \mu^B = 2.29$  in units of the nearest-neighbor hopping is found to maximize the HI band gap and may be realized by fine-tuning the above parameters.

To realize the  $xy$ -plane Floquet modulation  $i$ ), we propose to form a 2D standing wave of laser light centered on the odd sites of the lattice with intensity modulated in time. The energy shifts of the  $|1,0\rangle_A$  and  $|1,1\rangle_B$  states can be made equal by tuning the polar angle of the light's polarization to  $\theta = .96$  rad, owing to the anisotropic polarizability of  $^{40}\text{K}^{87}\text{Rb}$  [13]. An additional stationary standing wave on the even sites cancels the site-dependent non-zero average of the modulation, which is necessary to preserve translation invariance in the effective Hamiltonian. With a modulation frequency of  $\Omega_{xy} = 500$  Hz, we choose an intensity modulation of strength  $11 \times 10^{-3}$  kW/cm<sup>2</sup> to generate an energy modulation of  $\mu_{A,\mathbf{v}}^{xy} = 1.218\Omega_{xy}(-1)^{v_x+v_y} \sin(\Omega_{xy}t)$ . An additional space-independent modulation by the two beams creates a slightly altered modulation on the  $B$  sublattice,  $\mu_{B,\mathbf{v}}^{xy} = \Omega_{xy}[(\mu_{A,\mathbf{v}}^{xy}/\Omega_{xy}) + 0.090 \sin(\Omega_{xy}t)]$ .

We now turn to the  $z$ -gradient Floquet modulation. We find that oscillating the detuning in a piecewise constant

manner according to:

$$\begin{aligned}\mu_{A,\mathbf{v}}^z(\Omega_z t)/\Omega_z &= \begin{cases} g_1 v_z & 0 < \Omega_z t \leq \phi_1 \\ g_2 v_z & \phi_1 < \Omega_z t \leq \phi_2 \\ g_3 v_z & \phi_2 < \Omega_z t \leq \pi \\ -\mu_{A,\mathbf{v}}^z(2\pi - \Omega_z t) & \pi < \Omega_z t \leq 2\pi \end{cases} \\ \mu_{B,\mathbf{v}}^z(\Omega_z t)/\Omega_z &= \begin{cases} g_1 v_z + g_1^{SL} & 0 < \Omega_z t \leq \phi_1 \\ g_2 v_z + g_2^{SL} & \phi_1 < \Omega_z t \leq \phi_2 \\ g_3 v_z + g_3^{SL} & \phi_2 < \Omega_z t \leq \pi \\ -\mu_{B,\mathbf{v}}^z(2\pi - \Omega_z t) & \pi < \Omega_z t \leq 2\pi \end{cases},\end{aligned}\tag{24}$$

with  $g_1 = -0.592$ ,  $g_2 = .097$ ,  $g_3 = 1.091$ ,  $g_1^{SL} = .671$ ,  $g_2^{SL} = -.438$ ,  $g_3^{SL} = 1.710$ ,  $\phi_1 = .157$ ,  $\phi_2 = 1.794$ , maximizes the HI band gap. We calculate the electric field and AC light field gradients that give rise to this modulation. For a modulation of frequency  $\Omega_z = 5$  kHz (much larger than that of the  $xy$  modulation), we require an electric field gradient of order  $\delta E/\delta z \sim 1$  kV/cm<sup>2</sup>. With detunings of order  $\Delta\nu \sim 1 - 2$  GHz, and hence AC polarizabilities of order  $\alpha/h \sim 1$  kHz/(W/cm<sup>2</sup>), this leads to a required intensity gradient  $\delta I/\delta z \sim 5$  W/( $\mu\text{m cm}^2$ ). We propose to realize the gradient using the natural spreading of a Gaussian beam along its propagation axis. For a beam propagating along the  $z$ -direction, this spreading gives rise to a  $z$ -dependent intensity  $I(z) \sim A/z^2$  [15], and so a corresponding gradient  $\delta I(z)/\delta z \sim A/r^3 \sim I(z)/z$ . With a beam radius  $z \sim 100 \mu\text{m}$ , the desired gradient can be achieved with a modest intensity  $I \sim .5$  kW/cm<sup>2</sup> and power  $P \sim I(z) \times z^2 \sim 50$  mW.

Finally, we briefly comment on the feasibility of optically addressing single molecules, for use in probing the existence of edge modes in the Hopf insulator. We note that, for polar molecules separated by a distance of  $1 \mu\text{m}$ , Ref. [16] estimated that a beam of radius  $1 \mu\text{m}$  with reasonable power  $10 \mu\text{W}$  was sufficient to allow single-molecule addressing of the  $|0, 0\rangle \rightarrow |1, 0\rangle$  transition.

- 
- [1] N. Y. Yao, A. V. Gorshkov, C. R. Laumann, A. M. Läuchli, J. Ye, and M. D. Lukin, Physical review letters **110**, 185302 (2013).
  - [2] J. M. Brown and A. Carrington, *Rotational spectroscopy of diatomic molecules* (Cambridge University Press, 2003).
  - [3] T. E. Lee, Physical Review A **94** (2016), 10.1103/PhysRevA.94.040701, arXiv: 1608.01326.
  - [4] J. E. Moore, Y. Ran, and X.-G. Wen, Physical Review Letters **101** (2008), 10.1103/PhysRevLett.101.186805, arXiv: 0804.4527.
  - [5] J. Kobayashi, K. Aikawa, K. Oasa, and S. Inouye, Phys. Rev. A **89**, 021401 (2014).
  - [6] S. Kotochigova and E. Tiesinga, Phys. Rev. A **73**, 041405 (2006).
  - [7] K. D. Bonin and V. V. Kresin, *Electric-Dipole Polarizabilities of Atoms, Molecules, and Clusters* (World Scientific, Singapore, 1997).
  - [8] A. J. Stone, *The Theory of Intermolecular Forces* (Clarendon Press, London, 1996).
  - [9] K. Alps, A. Kruzins, M. Tamanis, R. Ferber, E. A. Pazyuk, and A. V. Stolyarov, The Journal of Chemical Physics **144**, 144310 (2016).
  - [10] A. Pashov, O. Docenko, M. Tamanis, R. Ferber, H. Knöckel, and E. Tiemann, Phys. Rev. A **76**, 022511 (2007).
  - [11] S. Kotochigova, E. Tiesinga, and P. S. Julienne, Eur. Phys. J. D **31**, 189 (2004).
  - [12] S. Kotochigova and D. DeMille, Phys. Rev. A **82**, 063421 (2010).
  - [13] B. Neyenhuis, B. Yan, S. A. Moses, J. P. Covey, A. Chotia, A. Petrov, S. Kotochigova, J. Ye, and D. S. Jin, Physical Review Letters **109** (2012), 10.1103/PhysRevLett.109.230403, arXiv: 1209.2226.
  - [14] B. Yan, S. A. Moses, B. Gadway, J. P. Covey, K. R. A. Hazzard, A. M. Rey, D. S. Jin, and J. Ye, Nature **501**, 521 (2013).
  - [15] A. Yariv, *Optical electronics; 4th ed.*, The Holt, Rinehart and Winston series in electrical engineering (Saunders College Publ., Fort Worth, TX, 1991) international edition.
  - [16] J. P. Covey, L. De Marco, Ó. L. Acevedo, A. M. Rey, and J. Ye, New Journal of Physics **20**, 043031 (2018).
